# Supplementary material for: Talking by the numbers: Networks identify productive forum discussions
Source: arXiv:1802.08738 source file (2018-02-23)
Supplement: Supplementary file 1 [file Traxler_etal_CN_Supplemental.pdf]

# Supplemental Material

## I. GRADE AND CENTRALITY CORRELATIONS

Backbone extraction reduces the number of edges in a network [1, 2], which changes node centrality values. At each successively lower level of alpha (fewer edges retained), we recalculated Pearson correlations between final grade and the new values of PageRank, Target Entropy, and Hide. Additionally, we calculated the Kendall's tau rank correlation coefficient [3] to compare the centrality rank of each node in a backbone with its rank in the original network. This allows us to track whether the general centrality "power structure" of the original network is preserved, or whether the backbone extraction has substantially changed the estimation of which nodes are the most important.

Tables I, II, and III show these values for each semester. In semester 1, centrality/grade correlations quickly become non-significant as $\alpha$ decreases to 0.5 or 0.1. In the case of Hide, the direction of the correlation actually inverts (and becomes significant again) at $\alpha = 0.1$.

The centrality rank correlations, $\tau$, shed some light on this unexpected behavior of Hide. For both PageRank and Target Entropy, the rank order of nodes' centrality shows a positive but decreasing correlation as $\alpha$ decreases. This means that as links are removed from the network, the students who were originally most central would undergo some changes, but most would keep their "importance." On the other hand, starting with $\alpha = 0.1$, the $\tau$ coefficient for Hide becomes effectively zero and then negative. For $\alpha = 0.05$ or 0.01, nodes that had been high-Hide in the original network are now low-Hide. Thus, the backbone extraction process is highly disruptive to the calculation of Hide, a pattern which continues in Semesters 2 and 3. With the exception of the non-significant $\tau_H$ at $\alpha = 0.1$ in Semester 1, all $\tau$ correlation values have $p < 0.001$.

TABLE I. Semester 1 backbone correlations. Pearson correlations ($r$) between centrality and grade are listed with $p$-values for PageRank, Target Entropy, and Hide. Kendall's $\tau$ shows the centrality rank order correlations for each backbone compared to the original $\alpha = 1$ network.

| | Centrality/grade correlations | | | | | | Rank order correlations | | |
|---|---|---|---|---|---|---|---|---|---|
| $\alpha$ | $r_{PR}$ | $p_{PR}$ | $r_{TE}$ | $p_{TE}$ | $r_H$ | $p_H$ | $\tau_{PR}$ | $\tau_{TE}$ | $\tau_H$ |
| 1.00 | 0.18 | 0.04 | 0.29 | 0.00 | -0.27 | 0.00 | 1.00 | 1.00 | 1.00 |
| 0.50 | 0.17 | 0.06 | 0.26 | 0.00 | -0.00 | 0.97 | 0.95 | 0.88 | 0.79 |
| 0.10 | 0.09 | 0.31 | 0.16 | 0.08 | 0.23 | 0.01 | 0.72 | 0.59 | 0.03 |
| 0.05 | 0.08 | 0.40 | 0.10 | 0.24 | 0.05 | 0.56 | 0.66 | 0.47 | -0.35 |
| 0.01 | 0.02 | 0.78 | 0.05 | 0.57 | 0.18 | 0.05 | 0.48 | 0.31 | -0.45 |

Semesters 2 and 3 replicate these patterns in $\tau$. The $r$ values in Semester 2 are generally smaller than Semester 1 and not statistically significant. In Semester 3, Pearson correlations for PageRank and Target Entropy keep both their size and low $p$-values to lower $\alpha$ levels, but the Hide correlation again vanishes immediately.

TABLE II. Semester 2 extracted backbones, centrality correlations, and rank correlations between backbones and original network.

| | Centrality/grade correlations | | | | | | Rank order correlations | | |
|---|---|---|---|---|---|---|---|---|---|
| $\alpha$ | $r_{PR}$ | $p_{PR}$ | $r_{TE}$ | $p_{TE}$ | $r_H$ | $p_H$ | $\tau_{PR}$ | $\tau_{TE}$ | $\tau_H$ |
| 1.00 | 0.13 | 0.17 | 0.17 | 0.08 | -0.18 | 0.06 | 1.00 | 1.00 | 1.00 |
| 0.50 | 0.12 | 0.21 | 0.19 | 0.05 | -0.05 | 0.58 | 0.95 | 0.89 | 0.53 |
| 0.10 | 0.12 | 0.23 | 0.08 | 0.40 | 0.02 | 0.87 | 0.77 | 0.69 | -0.38 |
| 0.05 | 0.11 | 0.24 | 0.14 | 0.14 | 0.03 | 0.73 | 0.67 | 0.61 | -0.54 |
| 0.01 | 0.06 | 0.51 | 0.18 | 0.06 | 0.24 | 0.01 | 0.55 | 0.48 | -0.42 |

TABLE III. Semester 3 extracted backbones, centrality correlations, and rank correlations between backbones and original network.

| | Centrality/grade correlations | | | | | | Rank order correlations | | |
|---|---|---|---|---|---|---|---|---|---|
| $\alpha$ | $r_{PR}$ | $p_{PR}$ | $r_{TE}$ | $p_{TE}$ | $r_H$ | $p_H$ | $\tau_{PR}$ | $\tau_{TE}$ | $\tau_H$ |
| 1.00 | 0.34 | 0.00 | 0.28 | 0.00 | -0.31 | 0.00 | 1.00 | 1.00 | 1.00 |
| 0.50 | 0.34 | 0.00 | 0.28 | 0.00 | 0.04 | 0.66 | 0.94 | 0.88 | 0.65 |
| 0.10 | 0.33 | 0.00 | 0.34 | 0.00 | 0.11 | 0.25 | 0.82 | 0.72 | -0.34 |
| 0.05 | 0.26 | 0.01 | 0.24 | 0.01 | 0.23 | 0.02 | 0.71 | 0.60 | -0.54 |
| 0.01 | 0.21 | 0.03 | 0.32 | 0.00 | 0.18 | 0.06 | 0.59 | 0.45 | -0.44 |

## II. BACKBONE EXTRACTION CODE

Below is source code for the Locally Adaptive Network Sparsification (LANS) backbone extraction method. See Foti *et al.* [1] for algorithm details and pseudocode. The implementation here uses three functions: `fracwt` converts a weighted adjacency matrix into a fractional edge weight matrix; `Fmat` calculates the empirical CDF for each row of a fractional edge weight matrix, ($\hat{\mathbf{F}}(p_{ij})$ as defined by Foti *et al.* [1]); `LANS` combines those functions in a loop to generate the new backbone adjacency matrix.

```
## fracwt: Calculate the fractional edge weight matrix for a network
# Input a weighted adjacency matrix
# Outputs equivalent fractional edge weight matrix
fracwt <- function(wt) {
  P <- data.matrix(wt/rowSums(wt))
  P[is.na(P)] <- 0  # clear zeros (occur when rowSum=0, for isolates)
  return(P)
}

## Fmat: Calculate the empirical CDF for each row of an adjacency matrix
# Input an NxN matrix of fractional edge weights
# Outputs an NxN matrix of the empirical CDF for all present edges of each node
Fmat <- function(P) {
  P <- data.matrix(P) # Must use a matrix, not rows of data frames
  Ntot <- dim(P)[1]
  Fcdf <- matrix(data=0,nrow=Ntot,ncol=Ntot)
  for (i in 1:Ntot) {
    if (sum(P[i,])>0) {  # skip rows for isolates
      Frow <- ecdf(P[i,P[i,]>0])
      Fcdf[i,P[i,]>0] <- Frow(P[i,P[i,]>0])
    }
  }
  return(Fcdf)
}

## LANS: Perform backbone extraction
# Input: weighted adjacency matrix and p-value cutoff (alpha)
# Output: Extracted backbone matrix
LANS <- function(wt,alpha=0.05) {
  wt <- data.matrix(wt)
  Ntot <- dim(wt)[1]
  # initialize Pij to Sij/sum(Sik), extracted adjacency matrix to zero
  P <- data.matrix(fracwt(wt))  # Convert data frame to matrix for quantile function below
  A <- matrix(data=0,nrow=Ntot,ncol=Ntot)
  Fcdf <- Fmat(P)  # compute empirical CDF matrix
  for (i in 1:Ntot) {
    # If 1-F(pij) < alpha, keep edge ij
```

```
    jkeep <- (1-Fcdf[i,]) < alpha
    # if Pij > pa, set Aij = Sij (also set Aji = Sij if symmetric backbone)
    if (sum(jkeep) > 0) A[i,jkeep] <- wt[i,jkeep]  # non-isolates only
  }
  return(A)
}
```

The code is tested below on the "simple star" example network of Foti *et al.* [1, Fig. 2]. Five nodes are connected in a "star" configuration with weight 2 edges, with additional weight 1 edges linking the four non-central nodes (figure below, left). At $\alpha = 0.05$, LANS should remove the lower-weight edges, leaving only the star structure (figure below, right).

```
test1 <- matrix(data=c(0,1,0,1,2,1,0,1,0,2,0,1,0,1,2,1,0,1,0,2,2,2,2,2,0),nrow=5)
gtest1 <- graph.adjacency(test1,weighted=TRUE)
Atest1 <- LANS(test1)
backtest1 <- graph.adjacency(Atest1,weighted=TRUE)
par(cex=1.8)
plot.igraph(gtest1,edge.width=E(gtest1)$weight,vertex.size=10,vertex.label=NA)
plot.igraph(backtest1,edge.width=E(backtest1)$weight,vertex.size=10,vertex.label=NA)
```

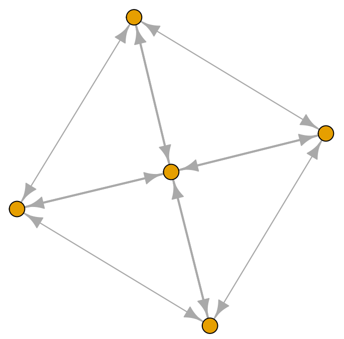

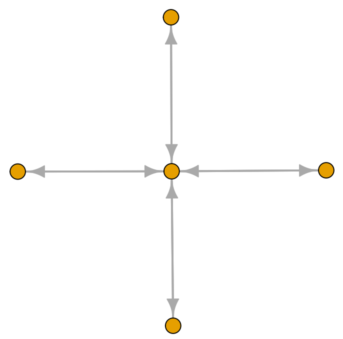


[1] Nicholas J. Foti, James M. Hughes, and Daniel N. Rockmore, "Nonparametric sparsification of complex multiscale networks," PLOS ONE **6**, e16431 (2011).

[2] M. Ángeles Serrano, Marián Boguñá, and Alessandro Vespignani, "Extracting the multiscale backbone of complex weighted networks," Proceedings of the National Academy of Sciences **106**, 6483–6488 (2009).

[3] Jean D. Gibbons, *Nonparametric Measures of Association*, Quantitative Applications in the Social Sciences No. 91 (SAGE, 1993).
